# Supplementary material for: Particles Prefer Walking Along the Axes: Experimental Insights into the Behavior of a Particle Swarm
Source: arXiv:1303.6145 source file (2013-08-08)
Supplement: Supplementary file 1 [file 06_appendix.tex]

\begin{appendix}

\section{Proof of Lemma \ref{run}}
\label{app:B}
\begin{proof}
Without loss of generality, assume that the swarm is positively running.
The main idea of this proof is to show that on expectation the energy increases after every step of the particle swarm.
More precisely, we want to show that $\E\left[1/\En_t^{n,d_0}\right]\xrightarrow{t\rightarrow\infty}0$,
which is equivalent to $1/\En_t^{n,d_0}\xrightarrow{t\rightarrow\infty}0$ almost surely and
therefore $\En_t^{n,d_0}\xrightarrow{t\rightarrow\infty}\infty$ almost surely.
Our strategy to prove the convergence of $\E\left[1/\En_t^{n,d_0}\right]$ is to prove that for
$\En_t^{n,d_0}\neq (0,0)$ the bound $\E\left[\En_t^{n,d_0}/\En_{t+1}^{n,d_0}\bigm| S_t\right] \le q$ holds for some fixed $q<1$ almost surely
(due to Lemma \ref{radoniko}, the case $\En_t^{n,d_0}= (0,0)$ for some $t$ has probability $0$).
This is sufficient because from there it follows
\begin{align*}
\lefteqn{\En_t^{n,d_0}\cdot\E\left[\frac{1}{\En_{t+k}^{n,d_0}}\bigm|S_t\right] = \E\left[\prod_{l=0}^{k-1} \frac{\En_{t+l}^{n,d_0}}{\En_{t+l+1}^{n,d_0}}\bigm|S_t\right]}\\
&= \E\left[\prod_{l=0}^{k-1} \hat{\En}_{t+l}\bigm|S_t\right]\\
\intertext{where we write $\hat{\En}_{t+l}$ for $\En_{t+l}^{n,d_0}/\En_{t+l+1}^{n,d_0}$. The $\hat{\En}_{t+l}$ are dependent,
so we cannot just look at the product of the single expectation values.
Instead we use the tower property of the conditional expectation (Thm. 5.1.6. in \cite{durrett2010probability}).}
&= \E\left[\E\left[\prod_{l=0}^{k-1} \hat{\En}_{t+l}\bigm|S_t,\hat{\En}_t\right] \bigm|S_t\right]\\
&= \E\left[\hat{\En}_t\cdot\E\left[\prod_{l=1}^{k-1} \hat{\En}_{t+l}\bigm|S_t,\hat{\En}_t\right] \bigm|S_t\right]\\
&= \E\left[\hat{\En}_t\cdot\E\left[\hat{\En}_{t+1}\cdot\E\left[\prod_{l=2}^{k-1} \hat{\En}_{t+l}\bigm|S_t,\hat{\En}_t,\hat{\En}_{t+1}\right] \bigm|S_t,\hat{\En}_t\right] \bigm|S_t\right]\\
&= \cdots\\
&= \E\left[\hat{\En}_t\cdot\E\left[\hat{\En}_{t+1}\cdot\ldots\E\left[\hat{\En}_{t+k-1}\bigm|S_t,\hat{\En}_t,\dots,\hat{\En}_{t+k-2}\right]\ldots\bigm|S_t,\hat{\En}_t\right] \bigm|S_t\right]\\
&= \E\left[\hat{\En}_t\cdot\E\left[\hat{\En}_{t+1}\cdot\ldots\E\left[\E\left[\hat{\En}_{t+k-1}\bigm|S_t,\ldots,S_{t+k-2}\right]\bigm|S_t,\hat{\En}_t,\ldots,\hat{\En}_{t+k-2}\right]\ldots\bigm|S_t,\hat{\En}_t\right] \bigm|S_t\right]\\
\intertext{Now we use the Markov property that $(\hat{\En}_t)$ inherits from $S_t$.}
&= \E\left[\hat{\En}_t\cdot\E\left[\hat{\En}_{t+1}\cdot\ldots\E\left[\E\left[\hat{\En}_{t+k-1}\bigm|S_{t+k-2}\right]\bigm|S_t,\hat{\En}_t,\ldots,\hat{\En}_{t+k-2}\right]\ldots\bigm|S_t,\hat{\En}_t\right] \bigm|S_t\right]\\
&\le \E\left[\hat{\En}_t\cdot\E\left[\hat{\En}_{t+1}\cdot\ldots\E\left[q\bigm|S_t,\hat{\En}_t,\ldots,\hat{\En}_{t+k-2}\right]\ldots\bigm|S_t,\hat{\En}_t\right] \bigm|S_t\right]\\
&= q\cdot\E\left[\hat{\En}_t\cdot\E\left[\hat{\En}_{t+1}\cdot\ldots\E\left[\hat{\En}_{t+k-2}\bigm|S_t,\hat{\En}_t,\ldots,\hat{\En}_{t+k-3}\right]\ldots\bigm|S_t,\hat{\En}_t\right] \bigm|S_t\right]\\
&\le \ldots \le q^k \xrightarrow{k\rightarrow\infty} 0
\end{align*}

The remaining part of the proof is rather technical.
We bound $\E\left[\En_t^{n,d_0}/\En_{t+1}^{n,d_0}\bigm| S_t\right]$ for our concrete choice of
energy from Def.~\ref{Energy}.
We know that there are better choices for the definition of an ``energy'' leading to larger
areas of parameters that match our requirements, but for our existence proof this one is sufficient.

We need to determine the values for $N$, $\chi$, $c_1$ and $c_2$, for which this energy fulfills 
\begin{equation}\label{APP:gewinn}
\E\left[\En_t^{n,d_0}/\En_{t+1}^{n,d_0}\bigm| S_t\right] \le q
\end{equation}
for a $q<1$. In other words, during one step of all particles, we want the reciprocal of the energy to decrease on expectation by at least a factor of $q$. This is granted if we can prove that the expectation during each step of a single particle is bounded from above by $1$ and that there is at least one particle with an expected decrease of the term bounded from above by $q$. Therefore we now focus only on the movement of one single particle $n$. If we can verify $\E[\En_t^{n,d_0} / \tilde{\En}_t^{n,d_0}]\le 1$ for every $n$ and $\E[\En_t^{n,d_0} / \tilde{\En}_t^{n,d_0}]\le q$ for at least one $n$, that would by the tower property of the conditional expectation imply (\ref{APP:gewinn}). We show the calculation only for particle $1$ since the situation is symmetric and we want to avoid too much mess with the indices.
\begin{align*}
\lefteqn{\E\left[\frac{\En_{t+1}^{1,d_0}}{\tilde{\En}_{t+1}^{1,d_0}}\bigm| S_t\right]}\\
&= \E\left[\sqrt{\frac{\sum_{n=1}^N a\cdot V_t^{n,d_0}+\left(G_{t+1}^{1,d_0}-X_t^{n,d_0}\right)}{a\cdot V_{t+1}^{1,d_0}+\left(\tilde{G}_{t+1}^{1,d_0}-X_{t+1}^{1,d_0}\right)+\sum_{n=2}^N a\cdot V_t^{n,d_0}+\left(\tilde{G}_{t+1}^{1,d_0}-X_t^{n,d_0}\right)}}\bigm| S_t\right]\\
\intertext{We substitute $\sum_{n=2}^N a\cdot V_t^{n,d_0}-X_t^{n,d_0}$ by $R$}
&= \E\left[\sqrt{\frac{a\cdot V_t^{1,d_0}+N\cdot G_{t+1}^{1,d_0}-X_t^{1,d_0}+R}{a\cdot V_{t+1}^{1,d_0}+N\cdot\tilde{G}_{t+1}^{1,d_0}-X_{t+1}^{1,d_0}+R}}\bigm| S_t\right]
\end{align*}
Now there are two distinct cases. In the first case, the position of particle $1$ is the global attractor, in terms $G_{t+1}^{1,d_0}=X_t^{1,d_0}$. Then its move is deterministic and its new position will be the new global attractor.
In this case, we obtain:
\begin{eqnarray*}
\lefteqn{\E\left[\frac{\En_{t+1}^{1,d_0}}{\tilde{\En}_{t+1}^{1,d_0}}\bigm| S_t\right] = \E\left[\sqrt{\frac{a\cdot V_t^{1,d_0}+(N-1)\cdot G_{t+1}^{1,d_0}+R}{a\cdot V_{t+1}^{1,d_0}+(N-1)\cdot\tilde{G}_{t+1}^{1,d_0}+R}}\bigm| S_t\right]}\\
&=&\sqrt{\frac{a\cdot V_t^{1,d_0}+(N-1)\cdot G_{t+1}^{1,d_0}+R}{a\cdot \chi\cdot V_t^{1,d_0}+(N-1)\cdot\left(G_{t+1}^{1,d_0}+\chi\cdot V_t^{1,d_0}\right)+R}}\\
&=&\sqrt{\frac{a\cdot V_t^{1,d_0}+(N-1)\cdot G_{t+1}^{1,d_0}+R}{(a+N-1)\cdot \chi\cdot V_t^{1,d_0}+(N-1)\cdot G_{t+1}^{1,d_0}+R}},
\end{eqnarray*}
which is less than $1$ for every possible $V_t^{1,d_0}$ and every possible $R$ if and only if $a<(a+N-1)\cdot \chi$. Given that, we can furthermore find the desired bound of a $q<1$, if $(N-1)\cdot\tilde{G}_{t+1}^{1,d_0}+R < \operatorname{const}\cdot V_t^{1,d_0}$ for some constant. That is the case, if particle $1$ has the largest value of $a\cdot V+(G-X)$ among all particles of the swarm and therefore makes the largest contribution to the energy.

The second case when $G_{t+1}^{1,d_0}>X_t^{1,d_0}$ is more difficult. Since the (modified) energy is invariant under translation, we can assume $X_t^{1,d_0}=0$. Furthermore, without loss of generality, we set $G_{t+1}^{1,d_0}=1$. Otherwise we could scale $\hat{\En}_t^1$ and $\tilde{L}_t^1$ by the factor $1/G_{t+1}^{1,d_0}$ and replace $V_t^{1,d_0} / G_{t+1}^{1,d_0}$ by $V_t^{1,d_0}$ and $R/G_{t+1}^{1,d_0}$ by $R$ which does not change the result since we need to bound the term for every positive $V_{t-1}^{1,d_0}$ and every $R>-(N-1)\cdot G_{t+1}^{1,d_0}$. We obtain:
\begin{align*}
\lefteqn{\E\left[\frac{\En_{t+1}^{1,d_0}}{\tilde{\En}_{t+1}^{1,d_0}}\bigm| S_t\right] = \E\left[\sqrt{\frac{a\cdot V_t^{1,d_0}+N\cdot G_{t+1}^{1,d_0}-X_t^{1,d_0}+R}{a\cdot V_{t+1}^{1,d_0}+N\cdot\tilde{G}_{t+1}^{1,d_0}-X_{t+1}^{1,d_0}+R}}\bigm| S_t\right]}\\
&=\E\left[\sqrt{\frac{a\cdot V_t^{1,d_0}+N+R}{a\cdot V_{t+1}^{1,d_0}+N\cdot\tilde{G}_{t+1}^{1,d_0}-X_{t+1}^{1,d_0}+R}}\bigm| S_t\right]\\
\intertext{Now we insert the movement equations of Def.~\ref{cPSO}}
&=\E\left[\sqrt{\frac{a\cdot V_t^{1,d_0}+N+R}{(a-1)\cdot \left(\chi\cdot V_t^{1,d_0}+c_2\cdot s_t^{1,d_0}\right)+N\cdot\max\left\{1,\chi\cdot V_t^{1,d_0}+c_2\cdot s_t^{1,d_0}\right\}+R}}\bigm| S_t\right]\\
&=\int_0^1 \sqrt{\frac{a\cdot V_t^{1,d_0}+N+R}{(a-1)\cdot \left(\chi\cdot V_t^{1,d_0}+c_2\cdot s\right)+N\cdot\max\left\{1,\chi\cdot V_t^{1,d_0}+c_2\cdot s\right\}+R}}\ ds\\
& =: I(\chi,c_2,N,a)
\end{align*}
Due to our choice of $\En$, the desired bound can be shown by extensive but straight-forward calculation, after eliminating the square roots a polynomial remains. We plotted the integral (see Figure \ref{Bild1}) %, \ref{Bild2} and \ref{Bild3}
for three different choices of the parameters, so one can easily verify that for the typical parameter sets found in the literature and a good choice for $a$, only two or three particles are sufficient to keep the value always less than $1$ and that under the assumption that particle $1$ makes the largest contribution to the modified energy, one can find an upper bound $\hat{q}<1$. Otherwise, another particle will satisfy that assumption and therefore lead to the desired bound. That finishes the proof.
\end{proof}

%\begin{figure}[htb]
%\centering
%\subfigure[$\chi = 0.729$, $c_2 = 1.49$, $N=2$, $a=2.69$ \cite{CK:02}]
%{\qquad\includegraphics[width=5cm,height=5cm]{chi=0p729c=1p49a=2p69N=2Fall2}\qquad}
%\subfigure[$\chi = 0.729$, $c_2 = 1.3\cdot \chi$, $N=3$, $a=5.38$ \cite{Carlisle01}]
%{\qquad\includegraphics[width=5cm,height=5cm]{chi=0p729c=1p3chia=5p38N=3Fall2}\qquad}
%\subfigure[$\chi = 0.6$, $c_2 = 1.7$, $N=3$, $a=2.98$ \cite{T:03}]
%{\quad\includegraphics[width=5cm,height=5cm]{chi=0p6c=1p7a=2p98N=3Fall2}\quad}
%\caption{\label{Bild1}The integral $I(\chi,c_2,N,a)$ for different parameter choices}
%\end{figure}

%\newpage

\section{Parameters satisfying Lemma \ref{run}}
\label{app:C}
\begin{figure}[htb]
\centering
\includegraphics[width=5cm,height=5cm]{Validparam}
\caption{\label{Validparam}Borders between the too low values for $c_2$ and $\chi$ and the ones large enough to satisfy the requirements in Lemma \ref{run} for some swarm sizes $N$.}
\end{figure}

\end{appendix}
